# Supplementary material for: Adding covariates to bounds: What is the question?
Source: arXiv:2502.03156 ancillary file (2025-03-25)
Supplement: Supplementary file 1 [file supplement.pdf]

# Adding covariates to bounds: What is the question—Supplementary Material

Gustav Jonzon      Erin E Gabriel      Arvid Sjölander  
Michael C Sachs

## 1 Proofs

*Proposition 2.* Uniform sharpness  $\Rightarrow$  Average bound sharpness:

$\{L_s : s \in \mathcal{S}\}$  is uniformly sharp if for all  $P_{\mathcal{O}} \in \mathcal{O}$  and all  $\varepsilon > 0$ , there exists a  $P_{\mathbf{V}} \in \bigcap_{s \in \mathcal{S}} o_s^{-1}(P_{\mathcal{O}|s})$  such that  $\theta_s(P_{\mathbf{V}}) < L_s(P_{\mathcal{O}|s}) + \varepsilon$  for all  $s \in \mathcal{S}$ , so  $\theta(P_{\mathbf{V}}) = \mathbb{E}_{P_{\mathbf{V}}}[\theta_S(P_{\mathcal{O}})] < \mathbb{E}_{P_{\mathbf{V}}}[L_S(P_{\mathcal{O}|S})] + \varepsilon = \bar{L}(P_{\mathcal{O}}) + \varepsilon$ , so  $\bar{L}(P_{\mathcal{O}})$  is sharp under  $G$ .

Uniform sharpness  $\Leftarrow$  Average bound sharpness:

For every  $\varepsilon > 0$  there exists a  $P_{\mathbf{V}}$  such that  $\int \theta_s(P_{\mathcal{O}}) dP_S(s) < \int L_s(P_{\mathcal{O}|s}) dP_S(s) + \varepsilon$ . Since  $\{L_s\}$  is valid,  $\theta_s(P_{\mathbf{V}}) \geq L_s(P_{\mathcal{O}|s})$  for almost every  $s \in \mathcal{S}$ . We want to show that  $\theta_s(P_{\mathbf{V}}) < L_s(P_{\mathcal{O}|s}) + \varepsilon$  for almost every  $s$ . Now we proceed by contradiction and suppose that there is a partition of  $\mathcal{S}$  into measurable sets  $A$  and  $B$  such that  $\theta_s(P_{\mathbf{V}}) \geq L_s(P_{\mathcal{O}|s}) + \varepsilon$  for  $s \in A$  and  $\theta_s(P_{\mathbf{V}}) < L_s(P_{\mathcal{O}|s}) + \varepsilon$  for  $s \in B$ . Since integration is order-preserving, we have

$$\begin{aligned} \int_A \theta_s(P_{\mathcal{O}}) dP_S(s) + \int_B \theta_s(P_{\mathcal{O}}) dP_S(s) &\geq \int_A L_s(P_{\mathcal{O}|s}) dP_S(s) + \int_B \theta_s(P_{\mathcal{O}}) dP_S(s) + \varepsilon \\ &\Rightarrow \\ \int \theta_s(P_{\mathcal{O}}) dP_S(s) &\geq \int_A L_s(P_{\mathcal{O}|s}) dP_S(s) + \int_B L_s(P_{\mathcal{O}|s}) dP_S(s) + \varepsilon = \\ &\int L_s(P_{\mathcal{O}|s}) dP_S(s) + \varepsilon \end{aligned}$$

which is a contradiction of the average bound sharpness. □

*Proposition 3.* From the definition of  $\theta_s$  we have that

$$\begin{aligned} \theta_s &= \sum_{y_0, x_0, x_1} p\{Y(X=0) = y_0, Y(X=1) = 1, X(Z=0) = x_0, X(Z=1) = x_1 | S = s\} \\ &- \sum_{y_1, x_0, x_1} p\{Y(X=0) = 1, Y(X=1) = y_1, X(Z=0) = x_0, X(Z=1) = x_1 | S = s\}. \end{aligned} \tag{1}$$

We further have that

$$\begin{aligned}
p(Y = y, X = x|S = s, Z = z) &= p\{Y(z) = y, X(z) = x|S = s, Z = z\} \\
&= p\{Y(z) = y, X(z) = x|S = s\} \\
&= p\{Y(x, z) = y, X(z) = x|S = s\} \\
&= p\{Y(x) = y, X(z) = x|S = s\} \\
&= \sum_{y', x'} p\{Y(x) = y, Y(1-x) = y', X(z) = x, X(1-z) = x'|S = s\},
\end{aligned} \tag{2}$$

where the first equality follows from consistency of counterfactuals, the second from Assumption 1, the third from consistency of counterfactuals, and the fourth from assumption 2. Thus, valid bounds on  $\theta_s$  are obtained by optimizing the right-hand side of (1), subject to the constraints on the distribution  $p\{Y(0), Y(1), X(0), X(1)|S\}$  defined by (2). Since this is precisely what Balke-Pearl optimization does, proposition 3 follows.  $\square$

## 2 Proposition 4

Note that some entries of  $A$  are actually independent of  $S$ .

We have  $A_1 = A_1^{-S}$ ,  $A_6 = A_6^{-S}$ ,  $A_{11} = A_{11}^{-S}$  and  $A_{16} = A_{16}^{-S}$  (by marginalizing out  $S$ ) so  $A^{-S} = \{A_1, A_6, A_{11}, A_{16}\} \subset A$  and the potential for covariate-assisted narrowing of the bounds resides entirely in the remaining 12 entries in  $A \setminus A^{-S}$ .

Again exploiting  $S \perp\!\!\!\perp Z$ , we get

$$\begin{aligned}
A &= \{p_{10.10} \cdot p_0 + p_{10.11} \cdot p_1, \\
&\quad -p_{00.00} \cdot p_0 - p_{01.00} \cdot p_0 + p_{10.10} \cdot p_0 + p_{01.10} \cdot p_0 + p_{10.11} \cdot p_1, \\
&\quad p_{10.00} \cdot p_0 + p_{01.00} \cdot p_0 - p_{00.10} \cdot p_0 - p_{01.10} \cdot p_0 + p_{10.11} \cdot p_1, \\
&\quad p_{10.00} \cdot p_0 + p_{10.11} \cdot p_1, \\
&\quad p_{10.10} \cdot p_0 - p_{00.01} \cdot p_1 - p_{01.01} \cdot p_1 + p_{10.11} \cdot p_1 + p_{01.11} \cdot p_1, \\
&\quad -p_{00.00} \cdot p_0 - p_{01.00} \cdot p_0 + p_{10.10} \cdot p_0 + p_{01.10} \cdot p_0 - p_{00.01} \cdot p_1 - p_{01.01} \cdot p_1 + p_{10.11} \cdot p_1 + p_{01.11} \cdot p_1, \\
&\quad p_{10.00} \cdot p_0 + p_{01.00} \cdot p_0 - p_{00.10} \cdot p_0 - p_{01.10} \cdot p_0 - p_{00.01} \cdot p_1 - p_{01.01} \cdot p_1 + p_{10.11} \cdot p_1 + p_{01.11} \cdot p_1, \\
&\quad p_{10.00} \cdot p_0 - p_{00.01} \cdot p_1 - p_{01.01} \cdot p_1 + p_{10.11} \cdot p_1 + p_{01.11} \cdot p_1, \\
&\quad p_{10.10} \cdot p_0 + p_{10.01} \cdot p_1 + p_{01.01} \cdot p_1 - p_{00.11} \cdot p_1 - p_{01.11} \cdot p_1, \\
&\quad -p_{00.00} \cdot p_0 - p_{01.00} \cdot p_0 + p_{10.10} \cdot p_0 + p_{01.10} \cdot p_0 + p_{10.01} \cdot p_1 + p_{01.01} \cdot p_1 - p_{00.11} \cdot p_1 - p_{01.11} \cdot p_1, \\
&\quad p_{10.00} \cdot p_0 + p_{01.00} \cdot p_0 - p_{00.10} \cdot p_0 - p_{01.10} \cdot p_0 + p_{10.01} \cdot p_1 + p_{01.01} \cdot p_1 - p_{00.11} \cdot p_1 - p_{01.11} \cdot p_1, \\
&\quad p_{10.00} \cdot p_0 + p_{10.01} \cdot p_1 + p_{01.01} \cdot p_1 - p_{00.11} \cdot p_1 - p_{01.11} \cdot p_1, \\
&\quad p_{10.10} \cdot p_0 + p_{10.01} \cdot p_1, \\
&\quad -p_{00.00} \cdot p_0 - p_{01.00} \cdot p_0 + p_{10.10} \cdot p_0 + p_{01.10} \cdot p_0 + p_{10.01} \cdot p_1, \\
&\quad p_{10.00} \cdot p_0 + p_{01.00} \cdot p_0 - p_{00.10} \cdot p_0 - p_{01.10} \cdot p_0 + p_{10.01} \cdot p_1, \\
&\quad p_{10.00} \cdot p_0 + p_{10.01} \cdot p_1\} \\
&= \{A_1^{|0} \cdot p_0 + A_1^{|1} \cdot p_1 \quad (= A_1^{-S}), \\
&\quad A_2^{|0} \cdot p_0 + A_1^{|1} \cdot p_1, \\
&\quad A_3^{|0} \cdot p_0 + A_1^{|1} \cdot p_1, \\
&\quad A_4^{|0} \cdot p_0 + A_1^{|1} \cdot p_1, \\
&\quad A_1^{|0} \cdot p_0 + A_2^{|1} \cdot p_1, \\
&\quad A_2^{|0} \cdot p_0 + A_2^{|1} \cdot p_1 \quad (= A_2^{-S}), \\
&\quad A_3^{|0} \cdot p_0 + A_2^{|1} \cdot p_1, \\
&\quad A_4^{|0} \cdot p_0 + A_2^{|1} \cdot p_1, \\
&\quad A_1^{|0} \cdot p_0 + A_3^{|1} \cdot p_1, \\
&\quad A_2^{|0} \cdot p_0 + A_3^{|1} \cdot p_1, \\
&\quad A_3^{|0} \cdot p_0 + A_3^{|1} \cdot p_1 \quad (= A_3^{-S}), \\
&\quad A_4^{|0} \cdot p_0 + A_3^{|1} \cdot p_1, \\
&\quad A_1^{|0} \cdot p_0 + A_4^{|1} \cdot p_1, \\
&\quad A_2^{|0} \cdot p_0 + A_4^{|1} \cdot p_1, \\
&\quad A_3^{|0} \cdot p_0 + A_4^{|1} \cdot p_1, \\
&\quad A_4^{|0} \cdot p_0 + A_4^{|1} \cdot p_1 \quad (= A_4^{-S})\} \\
&= \{p^0 \cdot p_0 + p^1 \cdot p_1 : p^0 \in A^{|0}, p^1 \in A^{|1}\} \\
&= A^{|0} \cdot p_0 + A^{|1} \cdot p_1 \quad (\text{Minkowski sum}) \\
&= \sum_{s \in \{0,1\}} A^{|s} \cdot p_s,
\end{aligned}$$

where we may split the original set into a sum of two sets since it consists precisely of all possible sums of elements of these two sets; note that all such combinations (and only such combinations) are present above. Thus we have

$$\begin{aligned}
L(P_{\mathbf{O}}) &= \max(A) && \text{(the covariate-optimal bound)} \\
&= \max(A^{|0} \cdot p_0 + A^{|1} \cdot p_1) \\
&= \max(A^{|0} \cdot p_0) + \max(A^{|1} \cdot p_1) && \text{(max distributes over Minkowski sums)} \\
&= \max(A^{|0}) \cdot p_0 + \max(A^{|1}) \cdot p_1 && \text{(since } p_0, p_1 \geq 0) \\
&= L_0(P_{\mathbf{O}|0}) \cdot p_0 + L_1(P_{\mathbf{O}|1}) \cdot p_1 && \text{(convex combination of the covariate-conditional bounds)} \\
&= \sum_{s \in \{0,1\}} L_s(P_{\mathbf{O}|s}) \cdot p_s \\
&= \bar{L}(P_{\mathbf{O}}) && \text{(the covariate-averaged bound).}
\end{aligned}$$

Thus the covariate-optimal and covariate-averaged lower bounds of  $\theta(P_{\mathbf{V}})$  coincide.

## 3 Simulation details

### 3.0.1 Objective

In planning the simulations, we follow the ‘‘ADEMP’’ structured approach proposed in [3]. This is a structured approach that entails specifying the following:

**Aims:** To evaluate methods for bounding causal effects in the presence of unmeasured confounding but where at least one measured covariate is available. We consider two main linear variations of IV settings with a categorical covariate, expressed via causal diagrams shown in Figure X. For each setting, we consider three methods of bounding the causal estimand: 1) computing sharp bounds on the ATE, 2) averaging bounds stratified by the measured covariate and 3) completely disregarding the measured covariate for comparison.

**Data-generating mechanisms:** Since bounds are generally used when unwilling to make further assumptions on the data-generating process, we will mainly make use of uniform sampling from the joint space of response function variables. As briefly reviewed in Notation and Methodology, their probabilities  $\mathbf{q}$  relate linearly to the observable conditional probabilities  $\mathbf{p}$ , through which our bounds are expressed, by  $\mathbf{q} = R\mathbf{p}$ . We may thus sample uniformly from the polytope  $P$  which constrains  $\mathbf{p}$  by uniformly sampling from the the simplex  $P$  of possible  $\mathbf{q}$ -values and mapping this space to  $P$  by  $R$ .

**Estimand / target of analysis:** Our target estimand is the population average causal risk difference, assuming a binary exposure as well as outcome. Apart from very special cases, this estimand will not be point-identifiable, but only interval-identifiable, in the settings we consider.

**Methods:** For baseline comparison, we will estimate bounds that ignore the additional covariate. The method we focus on evaluating is that of stratifying over the measured covariate, estimating bounds within its strata and averaging these to produce bounds. As a third method, we will using the general method of [4] to compute bounds on the setting that includes the covariate, but does not stratify over it.

**Performance measures:** There are several conceivable metrics to evaluate bounds: 1) the proportion that does not cover null (which is of most interest where stakes are high, as in medical contexts, e.g., 2) the width of the interval, and if the ground truth is known (as in simulations), 3) the proportion of valid bounds, i.e., contains the estimand (a crude metric but reassuring metric) as well as 4) how well the interval is centered around the estimand. To compare to sets of bounds, we will consider 1) (proper) inclusion, i.e., if one interval is properly contained within the other, and for more quantitative comparison, 2) the absolute difference in width and 3) the relative width as a proportion.

### 3.0.2 Simulation Methodology

Pseudocode for simulating covariate-optimal, covariate-marginalized, covariate-conditional and covariate-averaged bounds is shown below.

**Input:** A DAG  $D$  over the variables  $(S, Z, X, Y, U_r, U_l)$  where  $X, Y$  are binary,  $S, Z$  are categorical and  $U_r, U_l$  are latent.

**Output:** Covariate-optimal, covariate-marginalized and covariate-averaged bounds on  $\theta := \mathbb{E}[Y(X=1) - Y(X=0)]$  given  $D$  and a sampled observable distribution  $\mathbf{p}$ .

1. Sample a latent joint response function variable probability vector  $\mathbf{q}$  uniformly from the  $(k - 1)$ -simplex

$$\mathcal{Q} := \{\mathbf{q} \in [0, 1]^k : \|\mathbf{q}\| = 1\}$$

of all possible such values (a flat Dirichlet distribution) for  $U_r$  in  $D$ , where  $k$  is the number of distinct response functions of  $U_r$  in  $D$ .

2. Compute the corresponding value of the latent target estimand

$$\theta := \mathbf{c}^\top \mathbf{q}$$

, where  $\mathbf{c}$  is the gradient vector of the objective function guaranteed by the linearity of the optimization problem, and serves as a performance metric for the bounds.

3. If  $S \perp\!\!\!\perp Z$ , compute the corresponding observable conditional probability vector

$$\mathbf{p} := (p_{sxy.z} := P(S = s, X = x, Y = y | Z = z))_{s \in \mathcal{S}, z \in \mathcal{Z}, x \in \mathcal{X}, y \in \mathcal{Y}}$$

by

$$\mathbf{p} := R\mathbf{q}$$

, where  $R$  is the constraint matrix guaranteed by the linearity of the optimization problem, to get a sample  $\mathbf{p}$  from the polytope  $\mathcal{P}$  of all possible such values consistent with  $D$ .

If  $S \not\perp\!\!\!\perp Z$ , compute the corresponding observable conditional probability vector

$$\mathbf{p} := (p_{xy.zs} := P(X = x, Y = y | Z = z, S = s))_{s \in \mathcal{S}, z \in \mathcal{Z}, x \in \mathcal{X}, y \in \mathcal{Y}}$$

text by

$$\mathbf{p} := R\mathbf{q}$$

, where  $R$  is the constraint matrix

to get a sample  $\mathbf{p}$  from the polytope  $\mathcal{P}$  of all possible such values consistent with  $D$  and compute

$$\mathbf{p}_l := (p_{zs} := P(Z = z, S = s))_{s \in \mathcal{S}, z \in \mathcal{Z}}$$

by

$$\mathbf{p}_l := R_l \mathbf{q}_l$$

, where  $R_l$  is the constraint matrix corresponding to the left hand side and  $\mathbf{q}_l$  is a uniform sample of the response function variables probabilities corresponding to  $U_l$ , to get a sample  $\mathbf{p}_l$  from the polytope  $\mathcal{P}_l$  of all possible such values consistent with  $D$ .

**4.** Compute the covariate-optimal bounds

$$\mathbf{b}_{co}$$

from the covariate-optimal parameters  $\mathbf{p}$ . These bounds are guaranteed to be sharp given  $D$  and  $\mathbf{p}$ .

**5.** Compute the covariate-marginalized conditional probabilities

$$\mathbf{p}_{cm} := (p_{xy-z} := P(X = x, Y = y | Z = z))_{z \in \mathcal{Z}, x \in \mathcal{X}, y \in \mathcal{Y}}$$

by marginalizing out  $S$  from each entry of  $\mathbf{p}$ , aided by  $p_{sz}$  when  $S \not\perp Z$ .

**6.** Compute the covariate-marginalized bounds

$$\mathbf{b}_{cm}$$

from the covariate-marginalized parameters  $\mathbf{p}_{cm}$ . These bounds are guaranteed to be sharp given  $D \setminus \{S\}$  and  $\mathbf{p}_{cm}$ .

**7.** Compute the covariate marginal probabilities

$$\mathbf{p}_m := (ps := P(S = s))_{s \in \mathcal{S}}$$

by marginalizing out  $X$  and  $Y$  from each entry of  $\mathbf{p}$  and using  $S \perp\!\!\!\perp Z$  or marginalizing out  $Z$  from  $\mathbf{p}_l$  when  $S \not\perp Z$ .

**7.** Compute the covariate-conditional conditional probabilities

$$\mathbf{p}_{cc} := (\mathbf{p}_{cc,s} := (p_{xy-sz} := P(X = x, Y = y | S = s, Z = z))_{z \in \mathcal{Z}, x \in \mathcal{X}, y \in \mathcal{Y}})_{s \in \mathcal{S}}$$

by dividing each entry of  $\mathbf{p}$  by an entry of  $\mathbf{p}_m$  and using  $S \perp\!\!\!\perp Z$ .

**8.** Compute the covariate-conditional bounds

$$\mathbf{b}_{cc} := (\mathbf{b}_{cc}(s))_{s \in \mathcal{S}}$$

from the covariate-conditional parameters  $\mathbf{p}_{cc}$ .

**9.** Compute the covariate-averaged bounds

$$\mathbf{b}_{ca}$$

by convexly combining the covariate-conditional bounds  $\mathbf{b}_{cc}$  with the marginal probabilities  $\mathbf{p}_m$ .

**10.** Return

$$(\theta, \mathbf{b}_{cm}, \mathbf{b}_{ca}, \mathbf{b}_{co})$$

.

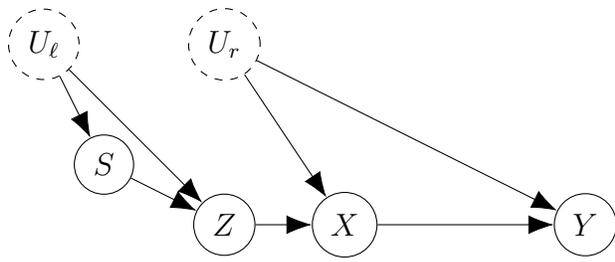

(a) Simulation setting 1

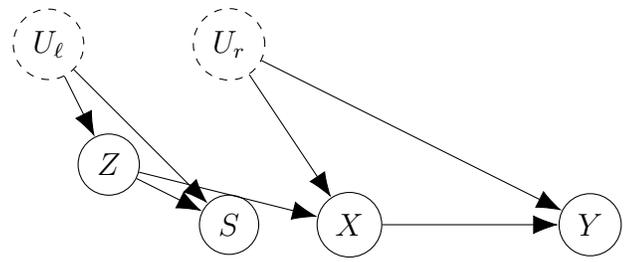

(b) Simulation setting 2

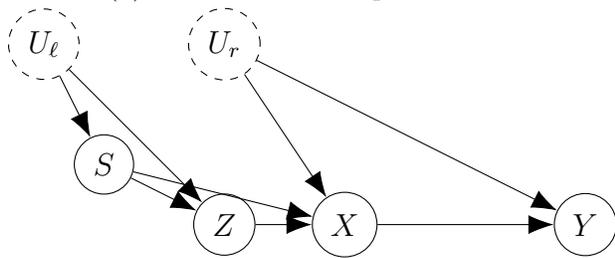

(c) Simulation setting 3

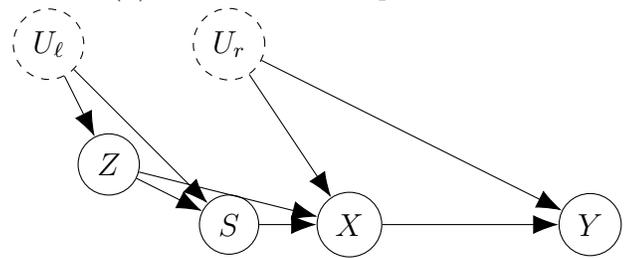

(d) Simulation setting 4

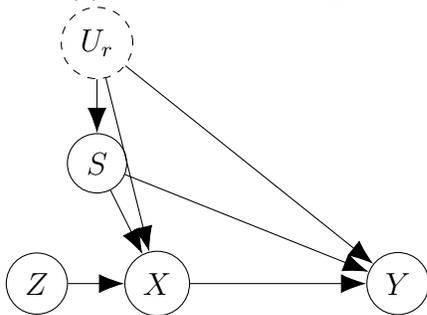

(e) Simulation setting 5

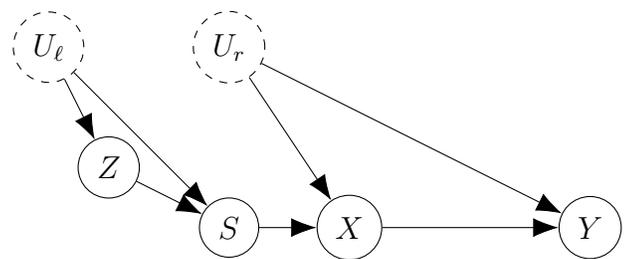

(f) Simulation setting 6

Figure 1: Simulation settings

### 3.0.3 Results

We performed  $n_{\text{sim}} := 10^5$  simulations for each of the following settings:

- a)  $S$  as a confounded parent of  $Z$  as shown in Figure 1a
- b)  $S$  as a confounded child of  $Z$  as shown in Figure 1b
- c)  $S$  as a confounded parent of  $Z$  and a parent of  $X$  as shown in Figure 1c
- d)  $S$  as a confounded child of  $Z$  and a parent of  $X$  as shown in Figure 1d
- e)  $S$  is independent of  $Z$  and confounded parent of  $X$  and  $Y$  as shown in Figure 1e
- f) The effect of  $Z$  on  $X$  is entirely mediated via  $S$

Each simulation setting used  $\mathcal{Z} := \{0, 1\}$  and  $\mathcal{S} := \{0, 1\}$ .

Each of these setting can be specialized by assuming some of the direct potential influences to be null. Some of these are considered in [1].

Table 1 shows summary statistics for each setting in Figure 1 and each set of bounds,

- cm: The covariate-marginalized bounds.
  - These bounds ignore the covariate, but are sharp given all information but the covariate.
  - They are referred to as covariate-agnostic in [2].
- ca: The covariate-averaged bounds.
  - These bounds are averages of covariate-conditional bounds within strata of the covariate.
  - Each covariate-conditional bound is sharp within its strata if global information on the covariate is inaccessible.
  - The covariate-averaged bounds are expected to be fully (but not necessarily properly) contained within the covariate-marginalized bounds.
  - They are referred to as covariate-assisted in [2].
- co: The covariate-optimal bounds.
  - These bounds are sharp given all information in its corresponding DAG, including global information on the covariate and are expected to be included within both of the above bounds.

using the following metrics, in the order they appear in the table:

- Validity: 1 if the bounds contain the partially identifiable estimand  $\theta = \mathbb{E}[Y(X=1) - Y(X=0)]$ .
  - This is a crude but essential metric. It is always expected to hold and in our context mostly serves as a sanity check.

- Null-coverage: 1 if the bounds contain 0.
  - This is significant in contexts where stakes are high and confidence that the effect of interest is bounded away from the null is desired.
  - In these settings, where the latent response function variable probabilities are sampled uniformly and without the latent constraints imposed in most naturally occurring settings, this is not expected to hold except for very rare occasions.
- Width: the difference in value between the upper and lower bound.
  - This is a natural target for minimization in a partial identifiability context, and a convenient metric by which to compare nested bounds.
- Distance from the midpoint of the bounds to its target estimand  $\theta$ .
  - Centering around the target estimand is another desirable feature. Although no assumption should be made regarding the distribution of the estimand within the bounds, this metric may detect interesting behaviour of the bounds.
- Inclusion, and especially proper inclusion, is the main qualitative relation of interest when comparing bounds.
  - We expect the chain of inclusions  $cm \subseteq ca \subseteq co$ , but these inclusions may not always be proper; we may very well have equalities for different settings.
  - Only once inclusion is established, width becomes a fair quantitative comparison metric, and the two in conjunction should be a preferable way to distinguish the performance of different bounds.

As expected and shown in Table 1, all bounds are valid but they almost always cover 0.

All three bounds coincide in the first two settings and are also the same across the two settings. This is expected, since they both essentially reduce to a single binary IV setting.

We always have the expected chain of inclusions across all settings except in models d and f, where the covariate-averaged bounds fail to be contained within the covariate-marginalized bounds, and for model f they are consistently worse. In model d, conditioning on  $S$  absorbs some of the effect of the IV rendering it a less effective IV, and in model f, it absorbs all of the effect rendering it useless as an IV.

In model c (Figure 1c), where  $S$  and  $Z$  are confounded joint binary IVs for  $(X, Y)$ , which is equivalent to a 4-level IV, these inclusions are both proper. That the covariate-marginalized bounds are inferior is due to it having access only to the binary IV  $Z$  with strictly less information than the IV  $(S, Z)$ , which provides more fine grained control of  $X$ .

The same phenomenon can be seen in model d (Figure 1d), where the connection between  $S$  and  $Z$  is reversed, but the combined interpretation is similar. Note that the covariate-marginalized bounds is the same in both of these settings. In setting d, however covariate-averaging fares worse than the covariate-marginalized bounds in almost half of the simulations.

Model e (Figure 1e) is the most general setting considered in [1], who showed the inclusion  $ca \subseteq cm$  and gave examples where this inclusion happens to be proper. These examples relied on different strata to distinguish different compliance rates  $Z \rightarrow X$ . It is noteworthy that

the covariate-averaged bounds coincide with the covariate-optimal bounds in this setting, whereas the inclusion of the covariate-marginalized bounds is proper, although it is nearly on par with the optimal bounds.

Model f violates the condition of [1], that  $S \perp\!\!\!\perp Z$ , as well as that of [2], that conditioning on  $S$  renders  $Z$  a valid instrument (since relevance/association is broken). The covariate-optimal bounds, however, are not affected and are furthermore strictly contained within the covariate-averaged bounds and of course the covariate-marginalized bounds.

## References

- [1] Zhihong Cai, Manabu Kuroki, and Tosiya Sato. “Non-parametric bounds on treatment effects with non-compliance by covariate adjustment”. In: *Statistics in Medicine* 26.16 (2007), pp. 3188–3204. DOI: <https://doi.org/10.1002/sim.2766>. eprint: <https://onlinelibrary.wiley.com/doi/pdf/10.1002/sim.2766>. URL: <https://onlinelibrary.wiley.com/doi/abs/10.1002/sim.2766>.
- [2] Alexander W Levis et al. “Covariate-assisted bounds on causal effects with instrumental variables”. In: *arXiv preprint arXiv:2301.12106* (2023).
- [3] Tim P. Morris, Ian R. White, and Michael J. Crowther. “Using simulation studies to evaluate statistical methods”. In: *Statistics in Medicine* 38.11 (2019), pp. 2074–2102. DOI: <https://doi.org/10.1002/sim.8086>. eprint: <https://onlinelibrary.wiley.com/doi/pdf/10.1002/sim.8086>. URL: <https://onlinelibrary.wiley.com/doi/abs/10.1002/sim.8086>.
- [4] Michael C. Sachs et al. “A General Method for Deriving Tight Symbolic Bounds on Causal Effects”. In: *JOURNAL OF COMPUTATIONAL AND GRAPHICAL STATISTICS* 32.2 (Apr. 2023), pp. 567–576. ISSN: 1061-8600. DOI: 10.1080/10618600.2022.2071905.

| metric                                              | model a | model b | model c | model d | model e | model f |
|-----------------------------------------------------|---------|---------|---------|---------|---------|---------|
| $\text{cm} \ni \theta$                              | 1.00    | 1.00    | 1.00    | 1.00    | 1.00    | 1.00    |
| $\text{ca} \ni \theta$                              | 1.00    | 1.00    | 1.00    | 1.00    | 1.00    | 1.00    |
| $\text{co} \ni \theta$                              | 1.00    | 1.00    | 1.00    | 1.00    | 1.00    | 1.00    |
| $\text{cm} \ni 0$                                   | 0.99    | 0.99    | 1.00    | 1.00    | 1.00    | 1.00    |
| $\text{ca} \ni 0$                                   | 0.99    | 0.99    | 1.00    | 1.00    | 1.00    | 1.00    |
| $\text{co} \ni 0$                                   | 0.99    | 0.99    | 1.00    | 1.00    | 1.00    | 0.99    |
| $\text{width}(\text{cm})$                           | 0.81    | 0.81    | 0.93    | 0.92    | 0.96    | 0.95    |
| $\text{width}(\text{ca})$                           | 0.81    | 0.81    | 0.90    | 0.90    | 0.95    | 1.00    |
| $\text{width}(\text{co})$                           | 0.81    | 0.81    | 0.82    | 0.82    | 0.95    | 0.81    |
| $\text{midpoint}(\text{cm})$                        | 0.00    | 0.00    | 0.00    | 0.00    | 0.00    | 0.00    |
| $\text{midpoint}(\text{ca})$                        | 0.00    | 0.00    | 0.00    | 0.00    | 0.00    | 0.00    |
| $\text{midpoint}(\text{co})$                        | 0.00    | 0.00    | 0.00    | 0.00    | 0.00    | 0.00    |
| $ \text{midpoint}(\text{cm}) - \theta $             | 0.08    | 0.08    | 0.04    | 0.04    | 0.02    | 0.08    |
| $ \text{midpoint}(\text{ca}) - \theta $             | 0.08    | 0.08    | 0.04    | 0.04    | 0.02    | 0.09    |
| $ \text{midpoint}(\text{co}) - \theta $             | 0.08    | 0.08    | 0.04    | 0.04    | 0.02    | 0.08    |
| $\text{co} \subseteq \text{cm}$                     | 1.00    | 1.00    | 1.00    | 1.00    | 1.00    | 1.00    |
| $\text{co} \subseteq \text{ca}$                     | 1.00    | 1.00    | 1.00    | 1.00    | 1.00    | 1.00    |
| $\text{ca} \subseteq \text{cm}$                     | 1.00    | 1.00    | 1.00    | 0.56    | 1.00    | 0.00    |
| $\text{width}(\text{cm}) - \text{width}(\text{co})$ | 0.00    | 0.00    | 0.11    | 0.10    | 0.01    | 0.14    |
| $\text{width}(\text{ca}) - \text{width}(\text{co})$ | 0.00    | 0.00    | 0.08    | 0.08    | 0.00    | 0.19    |
| $\text{width}(\text{cm}) - \text{width}(\text{ca})$ | 0.00    | 0.00    | 0.03    | 0.02    | 0.01    | -0.05   |
| $\text{width}(\text{co})/\text{width}(\text{cm})$   | 1.00    | 1.00    | 0.88    | 0.89    | 0.99    | 0.85    |
| $\text{width}(\text{co})/\text{width}(\text{ca})$   | 1.00    | 1.00    | 0.91    | 0.91    | 1.00    | 0.81    |
| $\text{width}(\text{ca})/\text{width}(\text{cm})$   | 1.00    | 1.00    | 0.97    | 0.98    | 0.99    | 1.05    |

Table 1: Averages from simulations with models (a) to (f) for the covariate-marginalized bounds (cm), the covariate-averaged bounds (ca) and covariate-optimal bounds (co) of the following individual metrics of the interval: valid (contains estimand), contains null, width, midpoint, mid-distance to estimand, and the following relative metrics: co contained in cm, co contained in ca, ca contained in cm, width(co) - width(cm), width(co) - width(ca), width(ca) - width(cm), width(cm)/width(co), width(ca)/width(co) and width(ca)/width(cm).
